# Supplementary material for: Peak Estimation for Uncertain and Switched Systems
Source: arXiv:2103.13017 source file (2021-03-24)
Supplement: Supplementary file 1 [file extensions.tex]

\section{Extensions}
% \urg{Should this be included at all, or left for arxiv? pushing the 6-page limit}
\label{sec:extensions}

This section briefly covers possible extensions of the uncertain peak estimation method. These extensions are all compatible with each other, and can be combined if desired.

\subsection{Running and State Costs}
Section 5 of \cite{fantuzzi2020bounding} proposes a method to penalize a running cost as well as a state cost in peak estimation. If $J(t, x)$ is a running cost of a continuous-time system with (possibly time-varying) state cost $p(t, x)$, the augmented objective of problem \eqref{eq:peak_traj} would be,
\begin{equation}
    \min p(t, x) + \int_{t' = 0}^t {J(t', x(t \mid x_0, w, d(t')) dt'}
\end{equation}
The discrete-time augmented objective for a system with costs $(p(x), J(x))$ is,
\begin{equation}
    \min p(x) + \sum_{t' = 0}^t {J(x(t \mid x_0, w, d_{t'}) }
\end{equation}
The weak formulations in problem \eqref{eq:peak_meas_un} or \eqref{eq:peak_meas_un_disc} would then have an objective,
\begin{equation}
    \min \inp{p}{\mu_p} + \inp{J}{\mu}
\end{equation}

For a switched system with $N_s$ states, each state may optionally have a state cost $p_k(t, x)$ and possess a running cost $J_k(t, x)$. Each running cost $J_k(t, x)$ only accrues during times $t$ when the trajectory $x(t \mid x_0, w, d(t))$ is following dynamics $f_k$ inside region $X_k$. To handle this per-state costs, the peak measure $\mu_p$ may be split into switch-peak measures $\mu_{pk} \in \Mp{[0, T] \times X_k \times W}$ such that $\mu_{p} = \sum_k \mu_{pk}$. The weak-formulation objectives \eqref{eq:peak_meas_un_obj} or \eqref{eq:peak_meas_un_disc_obj} may then be replaced with,
\begin{equation}
    \textrm{max} \quad \sum_{k=1}^{N_s} \inp{p_{k}(t,x)}{\mu_{pk}} + \inp{J_k(t, x)}{\mu_k} \label{eq:compound_objective}
\end{equation}

Constraint \eqref{eq:peak_cont_un_flow} would have a $J_k$ term, 
\begin{align}&\forall (t, x, w, d) \in [0, T] \times X_k \times W \times \Delta: \quad \forall k \\
    & \qquad \Lie_{f_{0k}} v(t, x, w) + \textstyle \sum_{\ell} \zeta_{k \ell}(t, x, w, d) + J_k(t, x) \leq 0 \label{eq:peak_cont_un_flow_J}.
\end{align}
and constraint \eqref{eq:peak_cont_un_p} would be replaced with a $p_k$ term,
\begin{align}&\forall (t, x, w) \in [0, T] \times X_k \times W : \quad \forall k \\
    & \qquad v(t, x, w) \geq p_k(x) \label{eq:peak_cont_un_flow_p}.
\end{align}

Similarly, constraint \eqref{eq:peak_cont_disc_flow} for a  discrete system in would have a $J_k$ term,
\begin{align}
        & \forall (x, w, d) \in  X_k \times W \times \Delta: \quad \forall k \nonumber \\
    & \quad v(f_k(x), w) -v(x, w) + J_k(x)  \leq  \alpha
\end{align}
and constraint \eqref{eq:peak_cont_disc_p} is replaced by a $p_k$ term, 
\begin{align}&\forall (x, w) \in X_k \times W : \quad \forall k \\
    & \qquad v(x, w) \geq p_k(x) \label{eq:peak_cont_un_p_J}.
\end{align}

\subsection{Integral Constraints}
\urg{I would need to rewrite my sampler to do the integral constraints and/or fixed noise processes.}

% \subsection{Disturbance Characterization}
Properties of the disturbance $d(t)$ may be specified by moment constraints on the disturbance-occupation measure $\mu^d$ defined in \eqref{eq:occ_measure_d}.

For any polynomial $h(d) \in \R[d]$, the integral quantity $\int_{t=0}^T h(d(t)) dt$ may be reformulated as $\inp{h(d)}{\mu^d}$.
% As an example, the process $d(t)$ may be constrained to have unit $L_2$ norm by imposing that $ \inp{\norm{d}_2^2}{\mu} = 1$.
As an example, the $L_2$-norm of the process $d(t)$ along system trajectories is $\norm{d(t)}_2 = \sqrt{\mathbb{E}[\norm{d}_2^2]} =  \sqrt{\inp{\norm{d}_2^2}{\mu^d}}$. The noise process may be constrained to have unit $L_2$ norm by imposing the moment constraint $\inp{\norm{d}_2^2}{\mu^d} = 1$ on $\mu^d$. $L_p$ norms with rational $p > 1$ can be handled with liftings to higher powers \cite{alizadeh2003second}. The $L_1$ norm can be realized by splitting $d(t) = d_+(t) - d_-(t) \in \Delta$ for $d_+, d_- \in \R_+^{N_d}$, with an effective norm $ \norm{d(t)}_1 = \inp{d_+ + d_-}{\mu^d}$.
% the $L_2$-norm of the process $d(t)$ % may be set to a value $e$ by imposing that $\norm{d(t)}_2^2 = \inp{\norm{d}_2^2}{\mu} = e^2$. 
A set of $N_h$ disturbance constraints $\{\int_{t=0}^T h_i(d(t)) dt = e_i\}_{i=1}^{N_h}$ may be imposed by adding constraints to \eqref{eq:peak_meas_un}
\begin{equation}
\inp{h_i(d)}{\textstyle\sum_{k} \mu_{k}} = e_i \quad  \forall i = 1, \ldots, N_h \label{eq:peak_meas_un_int}\\
\end{equation}

The addition of these disturbance constraints forms new dual variables $\lambda \in \R^{N_h}$. The new objective replacing  \eqref{eq:peak_cont_un_obj} is, 
\begin{equation}
    \min_{\gamma \in \R} \quad \gamma + \sum_{i=1}^{N_h} \lambda_i e_i,
\end{equation}
and the flow constraint \eqref{eq:peak_cont_un_flow} becomes, 
\begin{equation}
\Lie_{f_{0k}} v(t, x, w) + \textstyle \sum_{\ell} \zeta_{k \ell} + \textstyle \sum_i \lambda_i h_i(d) \leq 0.
\end{equation}

The same process occurs for a discrete system, where the constraint $\sum_{t=0}^T h(d_t)$ is transformed into the occupation measure constraint $\inp{h}{\mu^d}$. The objective \eqref{eq:peak_cont_un_disc_obj} becomes,
\begin{equation}
    \min \quad \gamma - T \alpha  + \sum_{i=1}^{N_h} \lambda_i e_i,
\end{equation}
and the disturbance constrained discrete flow constraint of \eqref{eq:peak_cont_disc_flow} is,
\begin{equation}
    v(f_k(x), w) -v(x, w)  + \textstyle\sum_i \lambda_i h_i(d)  \leq  \alpha
\end{equation}

% \urg{state inflation, Lipschitz disturbances}
\subsection{Continuity}
Continuity structure may be imposed on the disturbance process $d(t)$ by adding new states to the system (state inflation). As an example, assume that $d(t) \in \Delta = [d_{min}, d_{max}] \in \R, \  \forall t \in [0, T]$ is a 1-dimensional time-varying disturbance process influencing a dynamical system $\dot{x} = f(t, x, d)$. The process $d(t)$ can change arbitrarily quickly in time and has no assumptions of continuity. A derivative (slew rate) constraint $\abs{d'(t)} \leq L$ for some $L \in [0, \infty)$ enforces $C^1$ continuity of the process $d(t)$. The derivative-constrained noise may be realized by adding a new state $y \in \Delta$ such that $x' = f(t, x, y)$ where $y$ is the current value of the disturbance process. The dynamics of $y$ are $y'(t) = d_1(t)$, where $d_1(t)$ is a time varying noise process in the domain $[-L, L]$.

% Two new disturbance processes $d_+(t), \ d_-(t) \in [0, L]$ describing the arbitrarily varying bounded derivatives of the original disturbance. The dynamics of  $y$ are a switched system to ensure that $y \in [d_{min}, d_{max}]$,
% \begin{equation}
% \label{eq:state_inflation}
%     y' = \begin{cases}d_+(t) & y \leq d_{min} \\
%     d_+(t) - d_-(t) & d_{min} \leq y \leq d_{max} \\ 
%     -d_-(t) & y \geq  d_{max}.
%     \end{cases}
% \end{equation}

% \urg{Implement this? Likely to see numerical issues

% I think this is actually a hybrid system, where $y = d_{min}$ and $y = d_{max}$ are guards. Another reason to work on peak estimation for hybrid systems (besides local measures and low-degree approximation). This continuity content should not be used in the paper.
% }

% \urg{Get rid of the $h$ and $\lambda$ terms from the rest of paper, put in here.}
