# Supplementary material for: Peak Estimation for Uncertain and Switched Systems
Source: arXiv:2103.13017 source file (2021-03-24)
Supplement: Supplementary file 2 [file linear_applications.tex]

\section{Linear Peak Applications}

\label{sec:linear_app}

This section reviews how peak estimation can be used to bound the maximum absolute value of the impulse response and control effort of MIMO systems.

\subsection{Maximizing Multiple Objectives}

The impulse response and maximum control described later in this section may be realized as linear peak estimation programs \eqref{eq:peak_traj_lin} maximizing $p(x) = \max_i p_i(x)$ for $i = 1, \ldots, N_p$. The objective $p(x)$ can be bounded by solving program \eqref{eq:peak_meas_lin} for each objective $p_i(x)$ yielding upper bounds $p_{id}$. The resultant  bound to $p(x)$ is the maximum upper bound such that $p_{d}^* = \max_{i} p_{id}^*$.

An alternative approach is to maximize $p(x)$ by splitting the peak measure $\mu_p$ as $\sum_{i} \mu_{pi}$. Each split measure satisfies $\mu_{pi} \in \Mp{[0, T] \times X \times W}$. The primal-dual terms of \eqref{eq:peak_meas_lin_obj} and \eqref{eq:peak_cont_lin_p} may be expressed as,
\begin{equation}
    \max \quad \sum_{i=1}^{N_p} \inp{p_i}{\mu_{pi}} \qquad \qquad \qquad v(t, x, w) \geq p_i(x) \quad \forall (t, x, w) \in [0, T] \times X \times W, \ \forall i = 1, \ldots, N_p
\end{equation}

Optimizing over each $p_i$ individually requires solving $N_p$ separate problems. Splitting the peak measure $\mu_p$ into $\sum_i \mu_{pi}$ adds $N_p - 1$ nonnegativity constraints to the original single problem. The max-$i$ and split problems have the same optimum in the infinite dimensional linear program. At a finite degree relaxation the split problem will generally result in a higher bound than the max-$i$, because there is a single $v$ rather than a separate $v$ for each $p_i$. The split problem may be more reasonable to use when there are a large number of measures $(\mu_k, \sigma_{k \ell}, \hat{\sigma}_{k \ell})$ that would otherwise need to be duplicated with max-$i$.

An absolute penalty $\abs{c x}$for some vector $c \in \R^{1 \times N_x}$ may be realized as a max multiple objective peak estimation problem with $p(x) = \max (c x, -cx)$. This expression would not result in an block-diagonalizable invariant semidefinite program, as the function $c(-x) \neq c(x)$. The squared objective $(cx)^2$ is invariant under the transformation $x \rightarrow -x$, and a bound $P^*$ for $\abs{cx}$ may be computed by taking the square root of the upper bound $P^{2*}$ for $(c x)$.
If all objective functions $p_i(x)$ are even (including squared absolute values) then the invariant structure from section \ref{sec:even} may be used to simplify split and max-$i$ LMIs.

\subsection{Impulse Response Analysis}

One application of peak estimation for linear systems is estimating the maximum absolute value of the impulse response across all input/output pairs of a MIMO system \cite{chesi2019computation, chesi2020peak}. 

\subsubsection{Problem Setup}
The system $\dot{x} = Ax + Bu, \ y = C x$ has $N_x$ states, $N_y$ outputs, and $N_u$ inputs. 
The following assumptions are made:
\begin{itemize}
    \item $A_k(t, x, w, d, b)$ is a matrix of size $N_x \times N_x$ for each state $k$,  and dynamics may be decomposed into matrices $\{A_{k \ell}\}$ by \eqref{eq:lin_dynamics_aff}.
    \item $B$ and $C$ are functions strictly of $w$.
\end{itemize}

Define $\{B_j(w)\}_{j=1}^{N_u}$ as the columns of $B$ and $\{C_i(w)\}_{i=1}^{N_y}$ as the rows of $C$ for $i = 1 \ldots N_y$. If the system starting at $x(0) = 0$ receives an impulse at channel $j: \ u = \delta_j$, then the state immediately following this impulse is $x(0^+) = B_j(w)$. The corresponding trajectory is $x_j(t) = x(t \mid x_0 = B_j(w), w, d(t), b(t))$ for a given switching sequence and $d(t), b(t)$. A mixed input $u = \sum c_j \delta_j$ for weights $c_j \in \R^{N_u}, \ \sum_{j=1}^{N_u} c_j = 1$ will result in a trajectory $x(t) = \sum_{j=1}^{N_u} c_j x_j(t \mid x_0 = B_j(w), w, d(t), b(t))$. The set of plausible initial conditions $X_0$ of an impulse response is the convex hull of $\{B_j(w)\}_{j=1}^{N_u}$ for all $w \in W$.

For an output $i$, let $P^{2*}_i$ be the maximum value of the function $(C_i(w) x)^2$ along trajectories starting from $X_0$ (max-$i$). The maximum absolute value of the impulse response $P^*$ may be found,
\begin{equation}
    P^* = \max_i \sqrt{P^{2*}_i}
\end{equation}

% \urg{work on this later}

Program \eqref{eq:peak_meas_lin} with convex and even objective $p(x) = (C_i(w) x)^2$ may be used to upper bound the value $P^{2*}_i$. The initial condition $x^j = B_j(w) \in X, \forall w \in W$ is a function of $w$, and problems \eqref{eq:peak_meas_lin} and \eqref{eq:peak_cont_lin} must be changed accordingly. The invariant initial measure $\mu_0$ of the Liouville \eqref{eq:peak_meas_lin_flow} has the form,
\begin{equation}
\label{eq:even_w_init}
    \frac{1}{2}\left(\sum_{j = 1}^{N_0} \delta_{t = 0} \otimes(B_j(w), w)_\# \mu_{wj} +\delta_{t = 0} \otimes (-B_j(w), w)_\# \mu_{wj}\right)
\end{equation}
% Constraint \eqref{eq:peak_meas_lin_flow} is replaced by,
% \begin{align}
%         & \mu_p = \textstyle\sum_{j = 1}^{N_0} \delta_{t = 0} \otimes (B_j(w), w)_\# \mu_{wj} + \textstyle\sum_{k} \pi^{txw}_\#\Lie_{A_{k0} x}^\dagger \mu_{k} + \pi^{txw}_\#\textstyle\sum_{k\ell} ((A_{k \ell} x) \cdot \nabla_x)^\dagger \sigma_{k \ell}, & \label{eq:peak_meas_lin_flow_w}
% \end{align}
and the $x_j$ in constraint \eqref{eq:peak_cont_lin_init} is substituted,
\begin{equation}
    \quad {\gamma} \geq \frac{1}{2}\left(v(0, B_j(w), w) - v(0, -B_j(w))\right) = v(0, B_j(w), w) \qquad \qquad \forall w \in W, \ j = 1, \ldots, N_u \label{eq:peak_cont_lin_init_w}\\
\end{equation}

\cite{chesi2020peak} details an extensive treatment of an LMI approach towards bounding the impulse response of linear system with polytopic uncertainty. The linear system may switch between $\dot{x} = A_k x + B_k u, \ y = C_k x$ where the $B$ and $C$ matrices are also switching. This setting may be considered as a case of impulse-response estimation with larger $B$ and $C$ matrices formed by concatenating the $B_k$ along columns and $C_k$ along rows. The extended system would have $N_u N_s$ inputs, $N_y N_s$ outputs, and $N_x$ states. This is a slight relaxation as initial inputs cannot be applied to more than one $B_k$ at once. 
Convexity of $(C_{kj} x)^2$ implies that the optimal trajectory will start from at least one pure input $u = B_{kj}$, so the optimum value does not change by combining inputs $B_k$ together.

\subsubsection{Examples}

\urg{figures and examples go here. Need to fix my code and manually set yalmip to do the invariant measures. I don't know if gloptipoly can automatically handle invariant measures/sign symmetries.}

% For each output $B_j/C_i$ the bound $p^{2*}_{ij}$ is the square of the maximum absolute value of the impulse response. This quantity may be computed by:

\subsection{Maximum Control}
Another problem is finding the maximum state-feedback control effort for a linear system, as treated in \cite{rotondo2020saturation}. Assume that a state feedback controller $u = Kx$ with rows $K_j$ is provided to the linear system $\dot{x} = Ax + Bu$. The closed loop dynamics are $\dot{x} = A^{c\ell} x = (A + B K)x$ with output $y = K x$. Finding the maximum control effort for trajectories starting at some initial set $X_0$ is a peak estimation task with objectives $p_i(x) = \abs{K_i x}$.

% Just like in impulse response estimation, the computed bound $p^* = \max_j p_j^{2*}$ is accumulated from all rows $K_j$ individually. 
% If $X_0$ is polytopic with $N_0$ vertices, the max-control problem on channel $j$ can be decomposed into $N_0$ separate problems based on the vertices of $X_0$. 

% All linear system programs in this section remain valid for switched systems $\dot{x} = A_k x$ where $X^k = X$. This is due to linearity in dynamics when a switching sequence is fixed \cite{chesi2019ltv}. Problem \eqref{eq:peak_meas_impulse} has $\mu = \sum_k \mu^k$ as in Section \ref{sec:uncertain_switch}, and Constraint \eqref{eq:peak_cont_impulse_f} has $\inp{\nabla_x v(x)}{ A_k x}$ for each $k$. The max-control program has closed-loop matrices $A^{c\ell}_k = A_k + B K$. 

% \subsection{Maximum Control Effort}

% The peak estimation problem can be simplified in the case of linear dynamics  Begin by considering $\dot{x} = f(x) = A x$ where $X_0$ is polytopic with vertices

% Solves the same task as . 

% This is the only comparable paper i've seen so far. Will need to look further.
