# Supplementary material for: Peak Estimation for Uncertain and Switched Systems
Source: arXiv:2103.13017 source file (2021-03-24)
Supplement: Supplementary file 3 [file linear_system.tex]

\section{Linear Systems}
\label{sec:linear}
% \urg{I'm not sure if this can be spun off into its own paper. If it stays, add it to the introduction. This should be formatted in a more rigorous fashion, it is currently written like my notes.}

The structure of linear systems may simplify the LMIs necessary to bound extreme values of $p(x)$. The specific linear-in-state dynamics considered in this section are,

\begin{equation}
\label{eq:lin_dynamics}
    \dot{x} = f(x) = A_k(t, w, d, b) x \qquad \qquad \textrm{switching with } X^k = X \ \forall  k = 1, \ldots, N_s.
\end{equation}
It is required that all switching subsystems are valid ($X^k = X$) to ensure linearity of dynamics in all $X$. Dynamics in \eqref{eq:lin_dynamics} may be expanded by box-affine structure into,
\begin{equation}
    \label{eq:lin_dynamics_aff}
    \dot{x} = A_k(t, w, d, b)x = A_{k0}(t, w, d) x + \textstyle\sum_{\ell = 1}^{N_b} b_\ell A_{k \ell}(t, w, d) x .
\end{equation}
The uncertain peak estimation to maximize a function $p(x)$ with dynamics in \eqref{eq:lin_dynamics_aff} over sets $([0, T], X_0, X, W, \Delta)$ may be accomplished by relaxing program \eqref{eq:peak_meas_un} to the finite degree \eqref{eq:peak_lmi_un}. It is assumed that the set $X$ is invariant with respect to trajectories starting from $X_0$ over the time horizon $[0, T]$. 

One common problem setting is when the initial set $X_0$ is a polytope formed by the convex hull of vertices $\{x^j\}_{j=1}^{N_0}$ where $N_0 \leq \infty$. Any $x_0 \in X_0$ be can be expressed as $\sum_{j=1}^{N_0} c_j x^j$ where the weights $c \in \R^{N_0}_+$ satisfy $\sum_{j=1}^{N_0} c = 1$. A trajectory starting at $x_0$ may be decomposed as $x(t \mid x_0, w, d(t)) = \sum_{j=1}^{N_0} c_j x(t \mid x^j, w, d(t))$ by linearity. The ground-truth peak estimation program with convex polytopic $X_0$ may be restated using linearity as,
\begin{align}
\label{eq:peak_traj_lin}
P^* = & \max_{t,\, c ,\,  w ,\,  d(t)}  p(\textstyle \sum_{j=1}^{N_0} c_j x(t \mid x^j, w, d(t))) &\\
& \dot{x}_k(t) = A_{k0}(t, w, d) x + \textstyle\sum_{\ell = 1}^{N_b} b_\ell A_{k \ell}(t, w, d) x & t \in [0, T] \nonumber \\
&d(t) \in \Delta, \ b(t) \in [0, 1]^{N_b} & t \in [0, T] \nonumber \\
& w \in W, \  c \in \R_+^{N_0}, \ \textstyle\sum_{j=1}^{N_0} c_j = 1. \nonumber
\end{align}

Further structure may be exploited by analyzing properties of the objective $p(x)$. Convexity of $p(x)$ implies that
$p(x(1-\lambda) + \lambda(y)) \leq (1-\lambda) p(x) + \lambda p(y), \ \forall x, y \in X, \lambda \in [0, 1]$ by Jensen's inequality. 
This inequality carries over to trajectories, 
\begin{equation}
    \label{eq:linear_convex}
    p(\sum_{j=1}^{N_x} c_j x(t \mid x^j, w, d(t))) \leq \sum_{j=1}^{N_x} c_j p(x(t \mid x^j, w, d(t))) \leq \max_{j} p(x(t \mid x^j, w, d(t))) \qquad \forall t \in [0, T]
\end{equation}
The maximum $P^*$ will therefore be attained at a trajectory starting at one of the corners $x^j$. Problem \eqref{eq:peak_traj_lin} can therefore be split up into $N_0$ problems each starting at point $x^j$ ($c_j = 1, c_{j' \neq j} = 0\}$ and returning bounds $P^*_j$. The final $P^*$ is the maximum $P^*_j$ over all $j$.

A more general structure to the objective is if $p(x)$ is even such that $p(x) = p(-x)$. The linear dynamics in \eqref{eq:lin_dynamics} are equivariant to the transformation $x \rightarrow -x$, as $A(-x) = -(Ax)$. The initial set $X_0$ may be freely chosen to be the convex hull of $\pm x^j$ because 
\begin{equation}
   p(x(t \mid -x^j, w, d(t)) = p(-x(t \mid x^j, w, d(t)) =  p(x(t \mid x^j, w, d(t)).
\end{equation}

% The peak estimation task to maximize a convex $p(x)$ along trajectories starting in $X_0$ in times $[0, T]$ following linear dynamics in \eqref{eq:lin_dynamics_aff} is equivalent by \eqref{eq:linear_convex} to the following program,

% 

% This section analyzes the peak estimation problem of maximizing an objective $p(x)$ over  dynamics $\dot{x} = f(x) = A_k(t, w, d, b) x$ where $A_k$ is the uncertain linear dynamics at switching state $k$. 
% The peak estimation problem can be simplified if $p(x)$ is an even function and $X_0$ is a convex polytope
% formed by the convex hull of vertices $\{x^j\}_{j=1}^{N_0}$ where $N_0 \leq \infty$, and $X$ is known to be an invariant set with respect to $X_0$.

% \subsection{Linear Peak Estimation Problem}
% \urg{convexity not needed, is a bonus. evenness is}
% The following analysis does not exploit affine uncertainty structure, and is general to arbitrary disturbance processes $d(t)$. Convexity of $p(x)$ implies $\forall t \in [0, T]$:

% The maximum value of $p(x)$ along trajectories will therefore be attained at  a vertex $x^j$ for some possibly non-unique $j$. 
% % This result can be specialized to switching and box-type uncertainties by the methods of Section \ref{sec:affine}. Assume that there exists matrices $A_{k \ell}(t, w, d)$ of size $N_x \times N_x$ such that the possibly switched linear dynamics may be expanded into,

\subsection{Linear Measure Program}
Let $\mu_{wj} \in \Mp{W}$ be measures distributed over the uncertain parameters $w \in W$ for each corner point $x^j$ with $j = 1, \ldots, N_0$. The mass $\inp{1}{\mu_wj}$ takes the place of the weight $c_j$
A measure relaxation of Problem \eqref{eq:peak_traj_lin} with variables $(\mu_p, \mu_{wj}, \mu_k, \sigma_{k\ell}, \hat{\sigma}_{k \ell})$ is,

% \urg{I forgot about uncertainty $w$. Need to add that, would require changing everything. The variable is no longer $c_j$ in $c_j (\delta_{t = 0} \otimes\delta_{x = x^j})$, it is now $\mu_{wj}$ in $\delta_{t = 0} \otimes\delta_{x = x^j} \otimes \mu_{wj}$.}

\begin{subequations}
\label{eq:peak_meas_lin}
\begin{align}
p^* = & \ \textrm{max} \quad \inp{p(x)}{\mu_p} & \label{eq:peak_meas_lin_obj} \\
    & \mu_p = \textstyle\sum_{j = 1}^{N_0} \delta_{t = 0} \otimes\delta_{x = x^j} \otimes \mu_{wj} + \textstyle\sum_{k} \pi^{txw}_\#\Lie_{A_{k0} x}^\dagger \mu_{k}  \nonumber&\\
    &\quad \, + \pi^{txw}_\#\textstyle\sum_{k\ell} ((A_{k \ell} x) \cdot \nabla_x)^\dagger \sigma_{k \ell} & \label{eq:peak_meas_lin_flow}\\
    & \textstyle\sum_{j=1}^{N_0} \inp{1}{\mu_{wj}} = 1& \label{eq:peak_meas_lin_prob}\\
    & \sigma_{k \ell} + \hat{\sigma}_{k \ell} = \mu_k &\forall k, \; \ell\label{eq:peak_meas_lin_cont}\\
    & \mu_{k}, \ \sigma_{k \ell}, \ \hat{\sigma}_{k \ell} \in \Mp{[0, T] \times X \times W \times \Delta} &\forall k, \; \ell\\
    & \mu_p \in \Mp{[0, T] \times X \times W} & \\
    & \mu_{wj} \in \Mp{W} & \forall j& \label{eq:peak_meas_lin_init}
\end{align}
\end{subequations}

Problem \eqref{eq:peak_meas_lin} is a specialization of problem \eqref{eq:peak_meas_un}. 
The initial measure is expressed in terms of the vertices $x^j$ as $\mu_0 = \sum_{j = 1}^{N_0} \delta_{t = 0} \otimes\delta_{x = x^j} \otimes \mu_{wj}$. 
The initial measure may be left unchanged as $\mu_0 \in \Mp{X_0 \times W}$ if desired, especially if $X_0$ has a large number of vertices. 
In case there are no uncertain parameters in the system, the variables $\mu_{wj} \in \Mp{W}$ may be replaced by nonnegative scalar weights $c_j \geq 0$. Constraint \eqref{eq:peak_meas_lin_prob} would then read that $\sum_{j=1}^{N_0} c_j = 1$.

% The objective \eqref{eq:peak_meas_lin_obj} involves a single peak measure $\mu_p$, because splitting up $\mu_p$ into the sum of measures $\mu_{pj}$ would be computationally inefficient as $N_0$ grows
\subsection{Linear Function  Program}

The Lagrangian of Program \eqref{eq:peak_meas_lin} is:
\begin{align}
    \label{eq:linear_lagrangian}
    L &= \inp{p(x)}{\mu_p} + \inp{v(t,x,w)}{\textstyle\sum_{j = 1}^{N_0} (\delta_{t = 0} \otimes\delta_{x = x^j} \otimes \mu_{wj}) + \textstyle\sum_{k} \Lie_{A_{k0} x}^\dagger \mu_{k}} \nonumber\\
    &+ \inp{v(t,x,w)}{\textstyle\sum_{k\ell}(A_{k \ell} \cdot \nabla_x)^\dagger \sigma_{k \ell} - \mu_p} + \textstyle \sum_{j=1}^{N_0} c_j \psi_j \\
    &+ \gamma(1 -\inp{1}{\mu_{wj}}) + \textstyle\sum_{k \ell} \inp{\zeta_{k \ell}(t, x, w, d)}{\mu_k - \sigma_{k \ell} - \hat{\sigma}_{k \ell} } \nonumber .
\end{align}
% (1 - \inp{1}{\mu_0})

The resultant infinite-dimensional linear function program formed by minimizing the Lagrangian in \eqref{eq:linear_lagrangian} with variables $(v, \gamma, \zeta)$ is,

\begin{subequations}
\label{eq:peak_cont_lin}
\begin{align}
    d^* = & \ \min_{\gamma \in \R} \quad \gamma \label{eq:peak_cont_lin_obj}\\
    & \forall w \in W: \quad \forall j\nonumber \\
    & \quad {\gamma} \geq {v(0, x^j, w)} &   \label{eq:peak_cont_lin_init}\\
    & \forall (t, x, w, d) \in [0, T] \times X \times W \times \Delta: \quad \forall k, \; \ell \nonumber \\
    & \quad \partial_t v(t, x, w) + (A_{k0} x) \cdot \nabla_x v(t, x, w) + \textstyle \sum_{\ell} \zeta_{k \ell}\leq 0 \label{eq:peak_cont_lin_flow}\\
    & \quad (A_{k\ell} x) \cdot \nabla_x v(t, x, w) \leq \zeta_{k \ell} \\
    & \forall (t, x, w) \in [0, T] \times X \times W: \nonumber \\
    & \quad v(t, x) \geq p(x) \label{eq:peak_cont_lin_p}  \\
    &v \in C^1([0, T]\times X \times W) \label{eq:peak_cont_lin_v} \\
    & \zeta_{k \ell} \in C_+([0, T]\times X \times W \times \Delta) \qquad \forall k, \; \ell.
\end{align}
\end{subequations}

% The variable $\psi$ is absorbed into the inequality constraint of \eqref{eq:peak_cont_lin_init}.
When there are no uncertain parameters $w$, constraint \eqref{eq:peak_cont_lin_init} is replaced by,
\begin{equation}
    \gamma \geq v(0, x^j) \qquad  \forall j = 1, \ldots, N_0
\end{equation}

\subsection{Even objective}
\label{sec:even}
Problem \eqref{eq:peak_meas_lin} may be modified to produce an invariant linear program if $p(x)$ is even. The initial measure $\mu_0$ may be replaced by, 
\begin{equation}
\label{eq:even_init}
\mu_0 = \sum_{j = 1}^{N_0} \delta_{t = 0} \otimes \frac{1}{2}(\delta_{x = x^j} + \delta_{x = -x^j}) \otimes \mu_{wj}.
\end{equation}
The initial measure remains a probability measure describing points that start at $x = \pm x^j$. The peak measure $\mu_p$ is likewise invariant, because if a point $x^*$ satisfies $p(x^*) = P^*$ then the negative $-x^*$ also reaches $p(-x^*)=P^*$. The (disturbance) occupation measures all inherit this invariant structure given that the initial measure $\mu_0$ is invariant.

Moment matrices of invariant measures may be block-diagonalized \cite{cimprivc2009sums, riener2013exploiting}. The sizes and multiplicity of the blocks are related to the symmetry group's irreducible representations. If a measure $\mu$ is invariant on the action $x \rightarrow -x$, then the moment $\E_\mu[x^\alpha t^\beta w^\gamma d^\delta]$ vanishes to zero whenever $\abs{\alpha}$ is odd. As an example, the $x_1$ moment of $\delta_{x^j} + \delta_{x=-x^j}$ is $x^j_1 + (-x^j_1) = 0$. Moment matrices $\M[y]$ of this type of invariant measure can be block-diagonalized into $\M^{odd}[y]$ and $\M^{even}[y]$. The rows (and columns) of $\M^{odd}[y]$ are indexed by multi-indices where $\abs{\alpha}$ is odd, while $\M^{even}[y]$ has even $\abs{\alpha}$. 

The full moment matrix $\M_d[y]$ at degree $d$ has size $\binom{n+d}{d}$. The sizes of the two blocks are,
\begin{equation}
    \M^{odd}_d[y]: \ \sum_{d' \textrm{ even}}^{d} \binom{n+d'-1}{d'} \qquad \qquad \M^{even}_d[y]: \ \sum_{d' \textrm{ even}}^{d} \binom{n+d'-1}{d'},
\end{equation}
which together add to $\binom{n+d}{d}$. All measures $(\mu_0, \mu_p, \mu_k, \sigma_{k \ell}, \hat{\sigma}_{k \ell}$ may have their moment matrices block-diagonalized in this fashion, reducing the size of the semidefinite constraint blocks in the LMI.
% All other measures will inherit this even symmetric structure with $x \rightarrow -x$ due to equivariance of dynamics.

The dual problem \eqref{eq:peak_cont_lin} may implement this symmetry by requiring that $v(t, x, w) = v(t, -x, w)$. In the SOS relaxation, $v$ would then be a member of the invariant ring of polynomials with respect to this group action. Such a $v$ has a decomposition into $v^{odd}(t, x, w) + v^{even}(t, x, w)$ as described previously. Constraint \eqref{eq:peak_cont_lin_init} is effectively unaffected, as it is replaced by the equivalent, 
\begin{equation}
    \forall w \in W, \ \forall j = 1, \ldots, N_0: \qquad \gamma \geq \frac{1}{2}(v(0, x^j, w) + v(0, -x^j, w)) = v(0, x^j, w)
\end{equation}
to match the initial measure \eqref{eq:even_init}.

The set of sum-of-squares invariant polynomials is $\sigma^{odd}(t, x, w) + \sigma^{even}(t, x, w)$ where $\sigma^{odd}, \  \sigma^{even}$ are each SOS \cite{gatermann2004symmetry}. Program \eqref{eq:peak_cont_lin} may accomodate the invariant structure by using the invariant decomposition when enforcing the SOS constraints \eqref{eq:peak_cont_lin_flow} - \eqref{eq:peak_cont_lin_p}. The semidefinite Gram matrices describing SOS polynomials $\sigma_d^{odd}, \  \sigma_d^{even}$ are dual to the moment matrices $\M^{odd}_d[y], \ \M^{even}_d[y]$.
