# Supplementary material for: Peak Estimation for Uncertain and Switched Systems
Source: arXiv:2103.13017 source file (2021-03-24)
Supplement: Supplementary file 4 [file prelim_lmi_peak.tex]

\subsection{Peak Estimation LMI}

\label{sec:peak_lmi}
The peak estimation problem \eqref{eq:peak_meas} may be approximated through a moment LMI.

Let $(y^0, y^p)$ represent moment sequences up to order $2d$ of the measures $\mu$, and $y$ be moment sequences up to order $2(d + \textrm{deg}(f) -1)$ of the occupation measure $\mu$.
The Liouville equation in \eqref{eq:peak_meas_flow} induces a linear relation between the moment sequences $(y^0, y, y^p)$ for the test function $x^\alpha t^\beta$,
\begin{equation}
\label{eq:liou_mom_lmi}
    \inp{x^\alpha t^\beta}{ {\delta_0 \otimes} \mu_0} + \inp{\Lie_f( x^\alpha t^\beta)}{\mu} - \inp{x^\alpha t^\beta}{\mu_p} = 0.
\end{equation}
The expression $\textrm{Liou}_{\alpha \beta}(y^0, y, y^p)$ is defined as this expression at the test function $x^\alpha t^\beta$.
The degree-$d$ moment-LMI relaxation of program  \eqref{eq:peak_meas} is, 
\begin{subequations}
\label{eq:peak_lmi}
\begin{align}
    p^*_d = & \textrm{max} \quad \textstyle\sum_{\alpha} p_\alpha y_{\alpha 0}^p. \label{eq:peak_lmi_obj} \\
    & \textrm{Liou}_{\alpha \beta}(y^0, y, y^p) = 0 \quad \textrm{by \eqref{eq:liou_mom_lmi}} \forall (\alpha, \beta) \in \N^{n+1}_{\leq 2d} \label{eq:peak_lmi_flow}\\
    & y^0_0 = 1 \\
    & \M_d(y^0), \M_d(y), \M_d(y^p) \succeq 0 \label{eq:peak_lmi_psd} \\
    &\M_{d - d_{0i}}(g_{0i} y^0) \succeq 0  \label{eq:peak_lmi_init} & &\forall i = 1, \ldots, N_c^0\\ 
    &\M_{d - d_i}(g_{i} y) \succeq 0 & & \forall i = 1, \ldots, N_c \label{eq:peak_lmi_peai} \\ 
    &\M_{d - d_i}(g_{i} y^p) \succeq 0 & &\forall i = 1, \ldots, N_c \\ 
    &\M_{d-2}(t(T-t)y),   \ \M_{d-2}(t(T-t)y^p) {\; \succeq \;} 0. \label{eq:peak_lmi_supp2}
\end{align}
\end{subequations}

The formulation in \eqref{eq:peak_lmi} assumes that $X = \{g_i(x)\geq 0 \mid \ i = 1, \ldots, N_c\}$ and $X_0 = \{g_{0i}(x)\geq 0 \mid \ i = 1, \ldots, N_c^0\}$ are both compact (Archimedean) basic semialgebraic sets. Constraints \eqref{eq:peak_lmi_psd}-\eqref{eq:peak_lmi_supp2} enforce that $(y^0, y, y^p)$ are moments corresponding to representing measures $\mu_0 \in \Mp{X_0}$ and $\mu, \mu_p \in \Mp{[0, T] \times X}$. These representing measures may not satisfy the infinite-dimensional Liouville equation in constraint \eqref{eq:peak_meas_flow}, only a finite number of induced Liouville constraints are included in \eqref{eq:peak_lmi_flow}. 

The upper bounds $p_d^*$ will tend towards $P^*$ as $d\rightarrow \infty$ given that $X_0$ and $[0, T] \times X$ are each compact. By theorem C.20 of \cite{lasserre2009moments}, the degree-$d$ LMI problem \eqref{eq:peak_lmi} is strongly dual to the degree-$d$ SOS relaxation of \eqref{eq:peak_cont}. This duality justifies the name Moment-SOS hierarchy, where the `hierarchy' is posed over increasing degree $d$.
