# Supplementary material for: Peak Estimation for Uncertain and Switched Systems
Source: arXiv:2103.13017 source file (2021-03-24)
Supplement: Supplementary file 5 [file conclusion.tex]

\section{Conclusion}

\label{sec:conclusion}

% \urg{Conclude the paper. Summarize the problem and important findings. Add some extensions and future work.}

The problem of peak estimation with uncertainty may be upper bounded with an infinite-dimensional LP in occupation measures, and approximated by a sequence of LMIs. Time-independent and time-dependent (including box, and switching) uncertainties  are incorporated into this measure framework for continuous and discrete systems. Specific application of this method towards the analysis of linear systems was discussed. Future work includes performing peak estimation with further specialized uncertainty structures.
